# Supplementary material for: Energy-Efficient Power Loading for OFDM-based Cognitive Radio Systems with Channel Uncertainties
Source: arXiv:1801.05353 source file (2019-02-08)
Supplement: Supplementary file 2 [file appendix_B.tex]

%\newpage
\section*{Appendix B\\Proof of Proposition 2}

Similar to $\mathbb{OP}1$, $\mathbb{OP}2$ is convex and it is solved by applying the KKT conditions. The Lagrangian function $\mathcal{L}_{\mathbb{OP}2}(\mathbf{p},\mathbf{y},\boldsymbol \lambda)$ is expressed as

\begin{IEEEeqnarray}{rcl}
\mathcal{L}_{\mathbb{OP}2}(\mathbf{p},\mathbf{y},\boldsymbol \lambda) &{} = {}& \sum_{\ell = 1}^{L} \alpha^{(\ell)} \sum_{i = 1}^{N} p_i \varpi_i^{(\ell)} - \left(1-\sum_{\ell = 1}^{L}\alpha^{(\ell)}\right) \sum_{i = 1}^{N} \log_2(1 + \gamma_i p_i) + \lambda_i \left[-p_i + y_i^2\right] \nonumber \\
&{} + {}& \lambda_{N+1} \left[\sum_{i = 1}^{N} p_i - P_{th}^{(m)} X^{(m)} + y_{N+1}^2 \right] \nonumber \\
&{} + {}& \sum_{\ell = 1}^{L} \lambda_{N+2}^{(\ell)} \left[\sum_{i = 1}^{N} p_i \varpi_i^{(\ell)} -  P_{th}^{(\ell)} X^{(\ell)} + (y_{N+2}^{(\ell)})^2 \right],
\end{IEEEeqnarray}
where $\mathbf{y} = \left[y_1^2, ..., y_{N+1}^2, (y_{N+2}^{(\ell)})^2 \right]^T$ and $\boldsymbol \lambda = \left[\lambda_1, ..., \lambda_{N+1}, \lambda_{N+2}^{(\ell)} \right]^T$, $\ell = 1, ..., L$, are the vectors of the slack variables and Lagrange multipliers of length  $N + L + 1$. The optimal solution is found when $\nabla \mathcal{L}_{\mathbb{OP}2}(\mathbf{p},\mathbf{y},\boldsymbol \lambda) = 0$, which yields
\begin{subequations}
\begin{IEEEeqnarray}{rcl}
\frac{\partial \mathcal{L}_{\mathbb{OP}2}}{\partial p_i} &{}={}& \sum_{\ell = 1}^{L} \alpha^{(\ell)} \varpi_i^{(\ell)} - \frac{1-\sum_{\ell = 1}^{L}\alpha^{(\ell)}}{\ln(2) (p_i + \gamma_i^{-1})} - \lambda_i + \lambda_{N+1} + \sum_{\ell = 1}^{L} \lambda_{N+2}^{(\ell)} \varpi_i^{(\ell)} = 0, \label{eq:OP_1_first_2} \\
\frac{\partial \mathcal{L}_{\mathbb{OP}2}}{\partial \lambda_i} &{}={}& - p_i + y_i^2 = 0, \\
\frac{\partial \mathcal{L}_{\mathbb{OP}2}}{\partial \lambda_{N+1}} &{}={}& \sum_{i = 1}^{N} p_i - P_{th}^{(m)} X^{(m)} + y_{N+1}^2 = 0, \\
\frac{\partial \mathcal{L}_{\mathbb{OP}2}}{\partial \lambda_{N+2}^{(\ell)}} &{}={}& \sum_{i = 1}^{N} p_i \varpi_i^{(\ell)} -  P_{th}^{(\ell)} X^{(\ell)} + (y_{N+2}^{(\ell)})^2 = 0, \\
\frac{\partial \mathcal{L}_{\mathbb{OP}2}}{\partial y_i} &{}={}& 2 \lambda_i y_i = 0, \label{eq:OP_1_5_2}\\
\frac{\partial \mathcal{L}_{\mathbb{OP}2}}{\partial y_{N+1}} &{}={}& 2 \lambda_{N+1} y_{N+1} = 0, \label{eq:OP_1_6_2}\\
\frac{\partial \mathcal{L}_{\mathbb{OP}2}}{\partial y_{N+2}} &{}={}& 2 \lambda_{N+2}^{(\ell)} y_{N+2}^{(\ell)} = 0. \label{eq:OP_1_last_2}
\end{IEEEeqnarray}
\end{subequations}
It can be seen that (\ref{eq:OP_1_first_2})--(\ref{eq:OP_1_last_2}) represent $3 N + 2 L + 2$ equations in the $3 N + 2 L + 2$ unknown components of the vectors $\mathbf{p}, \mathbf{y}$, and $\boldsymbol \lambda$. Equation (\ref{eq:OP_1_5_2}) implies that either $\lambda_i = 0$ or $y_i = 0$, (\ref{eq:OP_1_6_2}) implies that either $\lambda_{N+1} = 0$ or $y_{N+1} = 0$, and (\ref{eq:OP_1_last_2}) implies that either $\lambda_{N+2}^{(\ell)} = 0$ or $y_{N+2}^{(\ell)} = 0$. Hence, eight possible cases exist, as follows:

---\textit{Case 1}: Setting $\lambda_i = 0$ (i.e., $p_i > 0$), $\lambda_{N+1} = 0$ (i.e., $\sum_{i = 1}^{N} p_i < P_{th}^{(m)} X^{(m)}$), and $\lambda_{N+2}^{(\ell)} = 0$ (i.e., $\sum_{i = 1}^{N} p_i \varpi_i^{(\ell)} < P_{th}^{(\ell)} X^{(\ell)}$) results in the optimal solution on the form
\begin{IEEEeqnarray}{c}
p_i^* = \frac{1-\sum_{\ell = 1}^{L}\alpha^{(\ell)}}{\ln(2) \sum_{\ell = 1}^{L} \alpha^{(\ell)} \varpi_i^{(\ell)}} - \gamma_i^{-1}, \quad i = 1, ..., N. \label{eq:sol_op2_1}
\end{IEEEeqnarray}

---\textit{Case 2}: Setting $\lambda_i = 0$ (i.e., $p_i > 0$), $y_{N+1} = 0$ (i.e., $\sum_{i = 1}^{N} p_i = P_{th}^{(m)} X^{(m)}$), and $\lambda_{N+2}^{(\ell)} = 0$ (i.e., $\sum_{i = 1}^{N} p_i \varpi_i^{(\ell)} < P_{th}^{(\ell)} X^{(\ell)}$) results in the optimal solution on the form
\begin{IEEEeqnarray}{c}
p_i^* = \frac{1-\sum_{\ell = 1}^{L}\alpha^{(\ell)}}{\ln(2) \left(\sum_{\ell = 1}^{L} \alpha^{(\ell)} \varpi_i^{(\ell)} + \lambda_{N+1}\right)} - \gamma_i^{-1}, \quad i = 1, ..., N, \label{eq:sol_op2_2}
\end{IEEEeqnarray}
where $\lambda_{N+1}$ is calculated to satisfy $\sum_{i = 1}^{N} p_i^* = P_{th}^{(m)} X^{(m)}$.

---\textit{Case 3}: Setting $\lambda_i = 0$ (i.e., $p_i > 0$), $\lambda_{N+1} = 0$ (i.e., $\sum_{i = 1}^{N} p_i < P_{th}^{(m)} X^{(m)}$), and $y_{N+2}^{(\ell)} = 0$ (i.e., $\sum_{i = 1}^{N} p_i \varpi_i^{(\ell)} = P_{th}^{(\ell)} X^{(\ell)}$) results in the optimal solution on the form
\begin{IEEEeqnarray}{c}
p_i^* = \frac{1-\sum_{\ell = 1}^{L}\alpha^{(\ell)}}{\ln(2) \left(\sum_{\ell = 1}^{L} (\alpha^{(\ell)} + \lambda_{N+2}^{(\ell)}) \varpi_i^{(\ell)} \right)} - \gamma_i^{-1}, \quad i = 1, ..., N, \label{eq:sol_op2_3}
\end{IEEEeqnarray}
where $\lambda_{N+2}^{(\ell)}$ are calculated to satisfy $\sum_{i = 1}^{N} p_i \varpi_i^{(\ell)} = P_{th}^{(\ell)} X^{(\ell)}$, $\ell = 1, ..., L$.

---\textit{Case 4}: Setting $\lambda_i = 0$ (i.e., $p_i > 0$), $y_{N+1} = 0$ (i.e., $\sum_{i = 1}^{N} p_i = P_{th}^{(m)} X^{(m)}$), and $y_{N+2}^{(\ell)} = 0$ (i.e., $\sum_{i = 1}^{N} p_i \varpi_i^{(\ell)} = P_{th}^{(\ell)} X^{(\ell)}$) results in the optimal solution on the form
\begin{IEEEeqnarray}{c}
p_i^* = \frac{1-\sum_{\ell = 1}^{L}\alpha^{(\ell)}}{\ln(2) \left(\lambda_{N+1} + \sum_{\ell = 1}^{L} (\alpha^{(\ell)} + \lambda_{N+2}^{(\ell)}) \varpi_i^{(\ell)}  \right)} - \gamma_i^{-1}, \quad i = 1, ..., N, \label{eq:sol_op2_4}
\end{IEEEeqnarray}
where $\lambda_{N+1}$ and $\lambda_{N+2}^{(\ell)}$ are calculated to satisfy $\sum_{i = 1}^{N} p_i^* = P_{th}^{(m)} X^{(m)}$ and $\sum_{i = 1}^{N} p_i \varpi_i^{(\ell)} = P_{th}^{(\ell)} X^{(\ell)}$, respectively, $\ell = 1, ..., L$.

---\textit{Case 5}: Setting $y_i = 0$ (i.e., $p_i = 0$), $\lambda_{N+1} = 0$ (i.e., $\sum_{i = 1}^{N} p_i < P_{th}^{(m)} X^{(m)}$), and $\lambda_{N+2}^{(\ell)} = 0$ (i.e., $\sum_{i = 1}^{N} p_i \varpi_i^{(\ell)} < P_{th}^{(\ell)} X^{(\ell)}$) results in the optimal solution $p_i^* = 0$.

---\textit{Case 6}: Setting $y_i = 0$ (i.e., $p_i = 0$), $y_{N+1} = 0$ (i.e., $\sum_{i = 1}^{N} p_i = P_{th}^{(m)} X^{(m)}$), and $\lambda_{N+2}^{(\ell)} = 0$ (i.e., $\sum_{i = 1}^{N} p_i \varpi_i^{(\ell)} < P_{th}^{(\ell)} X^{(\ell)}$) is invalid as it implies that $p_i^* = 0$ which violates $\sum_{i = 1}^{N} p_i^* = P_{th}^{(m)} X^{(m)}$, $P_{th}^{(m)} \neq 0$.

---\textit{Case 7}: Setting $y_i = 0$ (i.e., $p_i = 0$), $\lambda_{N+1} = 0$ (i.e., $\sum_{i = 1}^{N} p_i < P_{th}^{(m)} X^{(m)}$), and $y_{N+2}^{(\ell)} = 0$ (i.e., $\sum_{i = 1}^{N} p_i \varpi_i^{(\ell)} = P_{th}^{(\ell)} X^{(\ell)}$) is invalid as it implies that $p_i^* = 0$ which violates $\sum_{i = 1}^{N} p_i \varpi_i^{(\ell)} = P_{th}^{(\ell)} X^{(\ell)}$, $P_{th}^{(\ell)} \neq 0$, $\ell = 1, ..., L$.

---\textit{Case 8}: Setting $y_i = 0$ (i.e., $p_i = 0$), $y_{N+1} = 0$ (i.e., $\sum_{i = 1}^{N} p_i = P_{th}^{(m)} X^{(m)}$), and $y_{N+2}^{(\ell)} = 0$ (i.e., $\sum_{i = 1}^{N} p_i \varpi_i^{(\ell)} = P_{th}^{(\ell)} X^{(\ell)}$) is invalid as it implies that $p_i^* = 0$ which violates $\sum_{i = 1}^{N} p_i^* = P_{th}^{(m)} X^{(m)}$, $P_{th}^{(m)} \neq 0$ and $\sum_{i = 1}^{N} p_i \varpi_i^{(\ell)} = P_{th}^{(\ell)} X^{(\ell)}$, $P_{th}^{(\ell)} \neq 0$, $\ell = 1, ..., L$.

Combining \textit{cases} 1 and 5 results in the optimal solution on the form
\begin{IEEEeqnarray}{c}
p_i^* = \left[\frac{1-\sum_{\ell = 1}^{L}\alpha^{(\ell)}}{\ln(2) \sum_{\ell = 1}^{L} \alpha^{(\ell)} \varpi_i^{(\ell)}} - \gamma_i^{-1}\right]^+, \quad i = 1, ..., N.
\end{IEEEeqnarray}

Combining \textit{cases} 2 and 5 results in the optimal solution on the form
\begin{IEEEeqnarray}{c}
p_i^* = \left[\frac{1-\sum_{\ell = 1}^{L}\alpha^{(\ell)}}{\ln(2) \left(\sum_{\ell = 1}^{L} \alpha^{(\ell)} \varpi_i^{(\ell)} + \lambda_{N+1}\right)} - \gamma_i^{-1}\right]^+, \quad i = 1, ..., N.
\end{IEEEeqnarray}

Combining \textit{cases} 3 and 5 results in the optimal solution on the form
\begin{IEEEeqnarray}{c}
p_i^* = \left[\frac{1-\sum_{\ell = 1}^{L}\alpha^{(\ell)}}{\ln(2) \left(\sum_{\ell = 1}^{L} (\alpha^{(\ell)} + \lambda_{N+2}^{(\ell)}) \varpi_i^{(\ell)}\right)} - \gamma_i^{-1}\right]^+, \quad i = 1, ..., N.
\end{IEEEeqnarray}

Combining \textit{cases} 4 and 5 results in the optimal solution on the form
\begin{IEEEeqnarray}{c}
p_i^* = \left[\frac{1-\sum_{\ell = 1}^{L}\alpha^{(\ell)}}{\ln(2) \left(\lambda_{N+1} + \sum_{\ell = 1}^{L} (\alpha^{(\ell)} + \lambda_{N+2}^{(\ell)}) \varpi_i^{(\ell)} \right)} - \gamma_i^{-1}\right]^+, \quad i = 1, ..., N.
\end{IEEEeqnarray} 

The solution $p_i^*$ satisfies the KKT conditions \cite{Boyd2004convex}, and, hence, it is an optimal solution.
